# Supplementary material for: Transfer Learning for Human Activity Recognition using Representational Analysis of Neural Networks
Source: arXiv:2012.04479 source file (2021-02-23)
Supplement: Supplementary file 2 [file appendix.tex]

@misc{Xavier,
author={{Nvidia}},
title={{Jetson Xavier NX Developer Kit}},
year={2014},
howpublished={\url{https://developer.nvidia.com/embedded/jetson-xavier-nx-devkit} accessed 29 Sep. 2020},
}

@misc{tensorflow2015-whitepaper,
title={{TensorFlow}: Large-Scale Machine Learning on Heterogeneous Systems},
url={http://tensorflow.org/},
note={Software available from tensorflow.org},
author={
    Mart\'{\i}n~Abadi and
    others},
  year={2015},
}

@article{zeiler2012adadelta,
  title={Adadelta: an adaptive learning rate method},
  author={Zeiler, Matthew D},
  journal={arXiv preprint arXiv:1212.5701},
  year={2012}
}

@misc{chollet2015keras,
  title={Keras},
  author={Chollet, Fran\c{c}ois and others},
  year={2015},
  howpublished={\url{https://keras.io}},
}
